# Supplementary material for: Suppression of Spin Transfer to $\Lambda$ Hyperon in Deep-Inelastic Scattering
Source: arXiv:2411.06205 source file (2025-06-12)
Supplement: Supplementary file 1 [file supplemental_material.pdf]

# Supplemental Material: Suppression of Spin Transfer to $\Lambda$ in Deep Inelastic Scattering

Xiaoyan Zhao,[1] Zuo-tang Liang,[1] Tianbo Liu,[1, 2, *] and Ya-jin Zhou[1, †]

[1] *Key Laboratory of Particle Physics and Particle Irradiation (MOE), Institute of Frontier and Interdisciplinary Science, Shandong University, Qingdao, Shandong 266237, China*

[2] *Southern Center for Nuclear-Science Theory (SCNT), Institute of Modern Physics, Chinese Academy of Sciences, Huizhou 516000, China*

## I. DIFFERENTIAL CROSS SECTIONS OF THE TARGET FRAGMENTATION

The general cross section for spin-1/2 hadron production in polarized semi-inclusive deep inelastic scattering (SIDIS) within the target fragmentation (TF) is expressed in terms of fracture functions (FrFs) as

$$\begin{aligned}\frac{d\sigma^{(\mathrm{TF})}}{dx dy d\zeta d^2\mathbf{P}_{hT}} = \frac{4\pi\alpha^2}{yQ^2}\sum_a e_a^2 \Bigg\{ (\frac{y^2}{2}-y+1)\Big[ & M_U^U + \lambda\lambda_h M_L^L + |S_\perp||S_{h\perp}|\cos(\phi_S-\phi_{S_h})\, M_T^T \\ & + |S_\perp||S_{h\perp}|\frac{\mathbf{P}_{h\perp}^2}{M_h^2}\left(\cos(2\phi-\phi_S-\phi_{S_h})+\cos(\phi_S-\phi_{S_h})\right) M_T^{Th} \\ & - |S_\perp|\frac{\mathbf{P}_{h\perp}}{M_h}\sin(\phi-\phi_S)\, M_T^{Uh} - |S_{h\perp}|\frac{\mathbf{P}_{h\perp}}{M_h}\sin(\phi-\phi_{S_h})\, M_U^{Th} \\ & + \lambda|S_{h\perp}|\frac{\mathbf{P}_{h\perp}}{M_h}\cos(\phi-\phi_{S_h})\, M_L^{Th} + \lambda_h|S_\perp|\frac{\mathbf{P}_{h\perp}}{M_h}\cos(\phi-\phi_S)\, M_T^{Lh}\Big] \\ + \lambda_e y(1-\frac{y}{2})\Big[ & \lambda\Delta M_L^U + \lambda_h\Delta M_U^L - |S_\perp||S_{h\perp}|\sin(\phi_S-\phi_{S_h})\Delta M_T^T \\ & - |S_\perp||S_{h\perp}|\frac{\mathbf{P}_{h\perp}^2}{M_h^2}\left(\sin(2\phi_h-\phi_S-\phi_{S_h})+\sin(\phi_S-\phi_{S_h})\right)\Delta M_T^{Th} \\ & + |S_\perp|\frac{\mathbf{P}_{h\perp}}{M_h}\cos(\phi-\phi_S)\,\Delta M_T^{Uh} + |S_{h\perp}|\frac{\mathbf{P}_{h\perp}}{M_h}cos(\phi-\phi_{S_h})\,\Delta M_U^{Th} \\ & - \lambda|S_{h\perp}|\frac{\mathbf{P}_{h\perp}}{M_h}\sin(\phi-\phi_{S_h})\,\Delta M_L^{Th} - \lambda_h|S_\perp|\frac{\mathbf{P}_{h\perp}}{M_h}\sin(\phi-\phi_S)\,\Delta M_T^{Lh}\Big]\Bigg\}, \end{aligned} \tag{1}$$

where the subscripts and superscripts $U$, $L$, and $T$ denote the unpolarized, longitudinally polarized, and transversely polarized states of the nucleon and the final-state hadron, respectively, while the superscript $h$ signifies the presence of factors proportional to the $P_{h\perp}$. Referring to the general parametrization of the SIDIS cross section, we obtain the structure functions expressed in terms of FrFs. Among all the structure functions, 16 of them receive nonvanishing contributions at the leading twist. Within the current fragmentation (CF) mechanism, 32 structure functions can have nonzero contributions at the leading twist, and explicit expressions are available in Refs. [1–3]. This observation indicates that certain azimuthal asymmetries are unique to either the CF or TF. Consequently, the measurement of azimuthal asymmetries absent in the CF offers a potential method to probe the TF contribution, and such measurements could be pursued in future experiments.

## II. UNPOLARIZED CROSS SECTIONS INCLUDING CF AND TF CONTRIBUTIONS

As the events from CF and TF mechanisms are not isolated at medium energy experiments, the direct influence of the TF contribution on the differential cross section or multiplicity, particularly on the shape of $x_F$ and $z$ dependence, is also of considerable interest. After integrating over the transverse momentum, the differential cross section is expressed as [4]

$$\frac{d\sigma^{(\mathrm{TFR})}}{dx dy d\zeta} = \frac{4\pi^2\alpha^2}{yQ^2}\sum_a e_a^2\Bigg\{(\frac{y^2}{2}-y+1)\left[M_U^U + \lambda\lambda_h M_L^L + S_\perp S_{h\perp}\cos(\phi_S-\phi_{S_h})\, M_T^T\right]$$

* Contact author: liutb@sdu.edu.cn
† Contact author: zhouyj@sdu.edu.cn

$$+\lambda_e y(1-\frac{y}{2})\left[\lambda\Delta M_L^U+\lambda_h\Delta M_U^L-S_\perp S_{h\perp}\sin(\phi_S-\phi_{S_h})\Delta M_T^T\right]\Big\}. \quad (2)$$

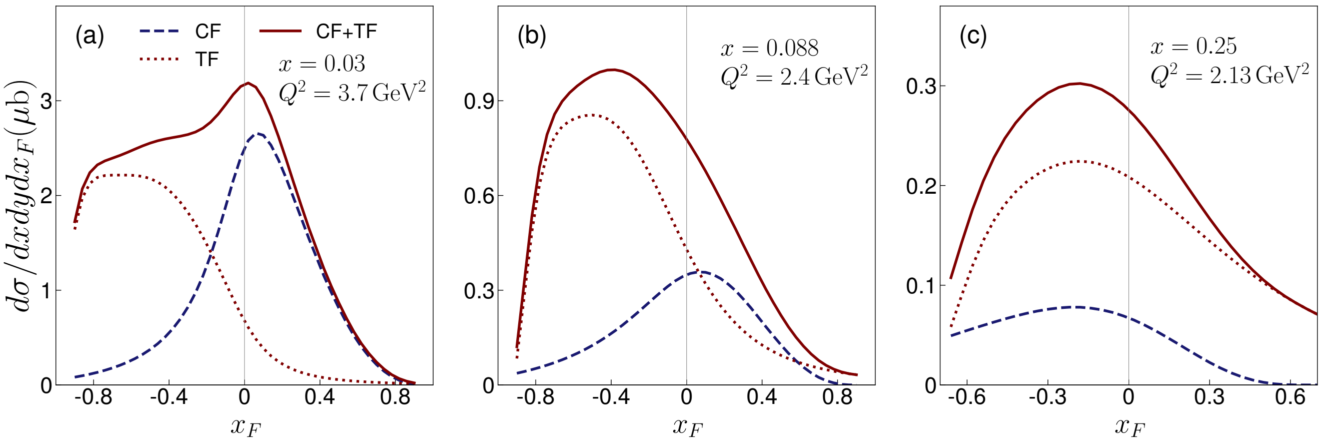


FIG. 1. Differential cross sections as a function of $x_F$.

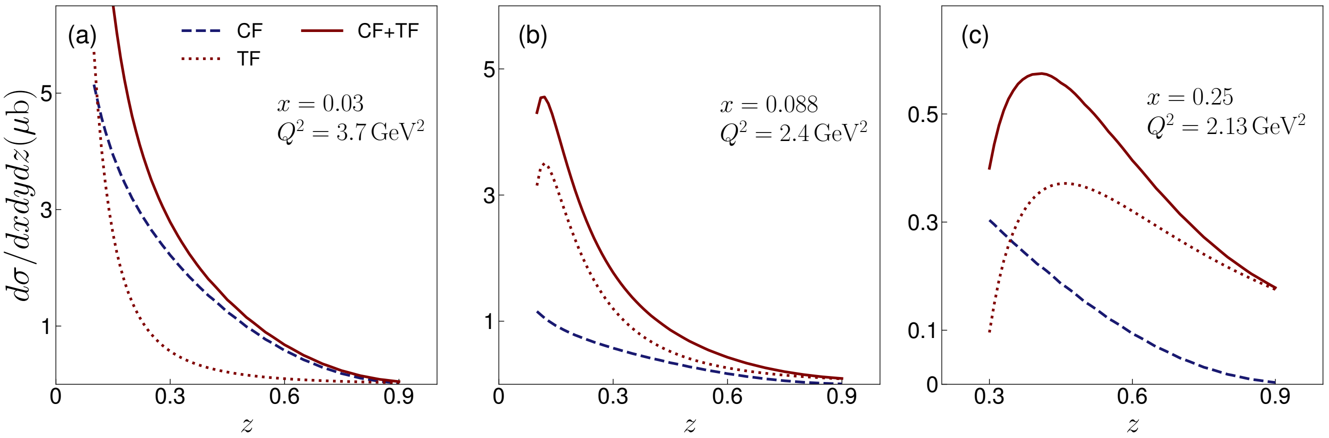


FIG. 2. Differential cross sections as a function of $z$.

In Figs. 1 and 2, we show the results of differential cross sections in $x_F$ and $z$ dependence, respectively, with other kinematic variables fixed according to the experimental conditions of COMPASS (a), HERMES (b), and CLAS (c). Dashed curves represent the CF contributions, dotted curves represent the TF contributions, and solid curves are the sum of CF and TF. As one can observe, the TF contribution is significant in low $x_F$ and $z$ regions, and its overall fraction increases at lower energies. This observation aligns with the findings from early neutrino experiments [5–11]. The calculation results further confirm the situation that no rapidity gap exists between CF and TF at these fixed target experiments. The TF may also play a crucial role in understanding the distributions of the produced $\Lambda$ hyperons.

## III. SPIN TRANSFER AT LARGE $x_F$

It is noteworthy that at large $x_F$, where the detected $\Lambda$ is along the virtual photon direction, the suppression effect of spin transfer $D_{LL}$ becomes even more significant. We note that $x_F$ is not an independent variable, at large-$x_F$ region, it corresponds to large $z$. In the CF, the struck quark needs to generate at least two pairs of quarks to form a $\Lambda$, which leads to the fall-off behavior of FF at large $z$ in powers of $(1-z)$. As the longitudinal momentum fraction increases, the $P_{h\perp}$ broadening is suppressed, consistent with observations in TMD studies, though not specifically for $\Lambda$ production. Consequently, the CF contribution at large $x_F$ rapidly drops with increasing $P_{h\perp}$. For the TF

contribution, large $x_F$ corresponds to small $\zeta$, meaning the generated $\Lambda$ carries only a small momentum fraction of the target remnant, leaving relatively more phase space for transverse momentum. Hence the TF contribution decreases slowly with increasing $P_{h\perp}$ in this region. Therefore, the spin transfer suppression effect by TF at the large-$x_F$ region becomes more pronounced with increasing $P_{h\perp}$.

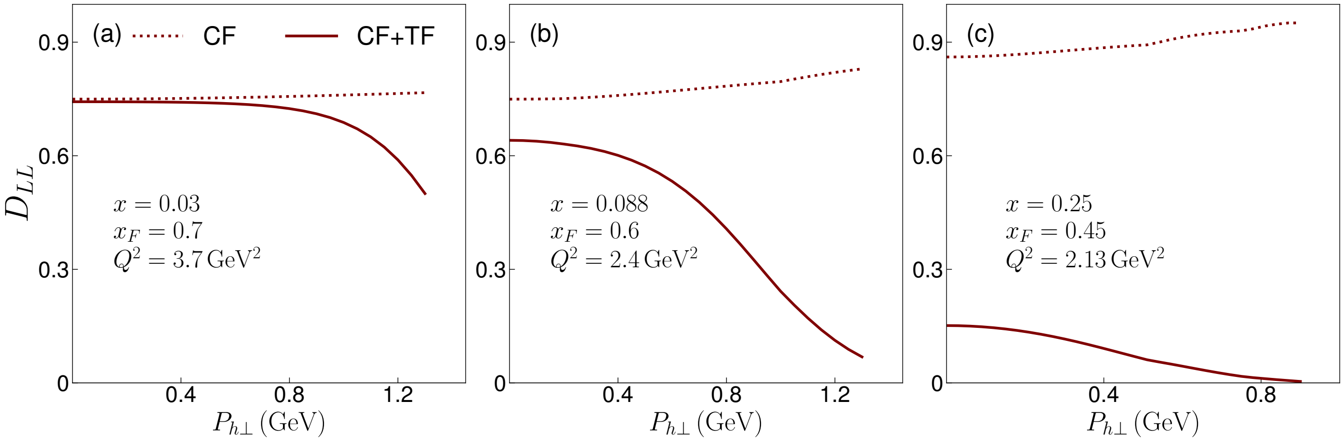


FIG. 3. $D_{LL}$ as a function of $P_{h\perp}$.

The $P_{h\perp}$ dependence of the spin transfer $D^{\Lambda}_{LL}$ at large-$x_F$ are shown in Fig. 3. The kinematic variables are chosen based on the coverage of COMPASS (a), HERMES (b), and CLAS (c) experiments at large $x_F$. One can observe that the TF contribution suppresses the spin transfer signal, particularly as $P_{h\perp}$ increases.


[1] D. Boer, R. Jakob and P. J. Mulders, Angular dependences in electroweak semi-inclusive leptoproduction, Nucl. Phys. **B564**, 471 (2000).

[2] A. Bacchetta, M. Diehl, K. Goeke, A. Metz, P. J. Mulders and M. Schlegel, Semi-inclusive deep inelastic scattering at small transverse momentum, J. High Energy Phys. 02 (2007) 093.

[3] J. Zhao, Z. Zhang, Z. t. Liang, T. Liu and Y. j. Zhou, Semi-inclusive production of spin-3/2 hadrons in deep inelastic scattering, Phys. Rev. D **109**, 074017 (2024).

[4] M. Anselmino, V. Barone, and A. Kotzinian, SIDIS in the target fragmentation region: Polarized and transverse momentum dependent fracture functions, Phys. Lett. B **699**, 108 (2011).

[5] V. V. Ammosov *et al.*, Charged current events with neutral strange particles in high-energy antineutrino interactions, Nucl. Phys. **B177**, 365 (1981).

[6] M. Arneodo *et al.* (The European Muon Collaboration), Quark and diquark fragmentation into neutral strange particles as observed in muon-proton interactions at 280 GeV, Phys. Lett. B **145**, 156 (1984).

[7] G. T. Jones *et al.* (Birmingham-Bonn-CERN-London-Munich-Oxford Collaboration), Polarization of $\Lambda$ hyperons produced inclusively in $\nu p$ and $\bar{\nu} p$ charged current interactions, Z. Phys. C **28**, 23 (1985).

[8] S. Willocq *et al.* (WA59 Collaboration), Neutral strange particle production in antineutrino-neon charged current interactions, Z. Phys. C **53**, 207 (1992).

[9] G. T. Jones *et al.* (WA21 Collaboration), Neutral strange particle production in neutrino and antineutrino charged current interactions on protons, Z. Phys. C **57**, 197 (1993).

[10] P. Astier *et al.* (NOMAD Collaboration), Measurement of the $\bar{\Lambda}$ polarization in $\nu_\mu$ charged current interactions in the NOMAD experiment, Nucl. Phys. **B605**, 3 (2001).

[11] D. DeProspo *et al.* (E632 Collaboration), Neutral strange particle production in neutrino and antineutrino charged-current interactions on neon, Phys. Rev. D **50**, 6691 (1994).
